# Supplementary material for: Estimates of the reproduction ratio from epidemic surveillance may be biased in spatially structured populations
Source: arXiv:2307.13798 source file (2025-01-07)
Supplement: Supplementary file 1 [file arxiv_SI_pdf.pdf]

# Contents

**1 Supplementary Methods** **2**

1.1 On the applicability of the Perron-Frobenius theorem . . . . . . . . . . . 2

1.2 Local estimated reproduction ratio . . . . . . . . . . . . . . . . . . . . . 3

1.2.1 Convergence . . . . . . . . . . . . . . . . . . . . . . . . . . . . 3

1.2.2 Decay modes . . . . . . . . . . . . . . . . . . . . . . . . . . . . 3

1.3 Estimation of department-level incident infections . . . . . . . . . . . . . 4

1.3.1 Models . . . . . . . . . . . . . . . . . . . . . . . . . . . . . . . 4

1.3.2 Comparison to seroprevalence data . . . . . . . . . . . . . . . . . 5

1.4 The stochastic epidemic model . . . . . . . . . . . . . . . . . . . . . . . 6

1.4.1 Reference reproduction ratio . . . . . . . . . . . . . . . . . . . . 7

1.4.2 Generation interval and EpiEstim settings . . . . . . . . . . . . . 8

1.5 Oscillations in European countries . . . . . . . . . . . . . . . . . . . . . 9

**2 Supplementary Figures** **10**

2.1 Decay time and oscillation period of the modes of $\Delta = R^{estim} - R^{ref}$ for selected European countries . . . . . . . . . . . . 10

2.2 Relative effect of the diagonal correction to co-location probabilities in French departments . . . . . . . . . . . . . . . . . . . . . . . . . . . 11

2.3 Daily number of new COVID-19-related infections per 100,000 residents 12

2.4 National attack rate: estimates vs serological studies . . . . . . . . . . . 14

2.5 Age demographic distribution in French regions . . . . . . . . . . . . . . 16

2.6 Fig. 1b and Fig. 4 of the main paper, using the age-stratified model for the estimate of infections . . . . . . . . . . . . . . . . . . . . . . . . . . . 17

2.7 Comparison of the reference, estimated and corrected reproduction ratios with six different initial conditions for the stochastic model . . . . . . . . 18

2.8 Comparison between point-wise medians and single runs of the stochastic metapopulation model . . . . . . . . . . . . . . . . . . . . . . . . . . 19

2.9 Variation of the spatial distribution of infections between weeks 6 and 11 of 2021, and the equilibrium distribution . . . . . . . . . . . . . . . . . . 21

**Supplementary References** **23**

# 1 Supplementary Methods

## 1.1 On the applicability of the Perron-Frobenius theorem

The Perron-Frobenius theorem as used in the main paper requires that the matrix be strictly positive ($R_{ij} > 0$), or nonnegative ($R_{ij} \geq 0$) and irreducible. In our case $R$ may not be strictly positive if, for some $i, j$, cases from $i$ generate no cases in $j$, so we shall prove here that it is irreducible, or that it can be made irreducible. A nonnegative matrix is irreducible if and only if its associated directed graph is strongly connected [1]. The associated graph of $R$ is that which has a link between nodes $i, j$ if $R_{ij} > 0$. In general, a suitable permutation of the node indices will bring $R$ to the following form, which mirrors the general bow-tie structure of the associated directed graph:

$$R = \left(\begin{array}{c|c|c} T_u & 0 & 0 \\ \hline B_1 & R_{scc} & 0 \\ \hline B_2 & B_3 & T_d \end{array}\right). \tag{S1}$$

where the blocks $T_u, T_d$ are lower diagonal and $R_{scc}$ is the adjacency submatrix of strongly connected component. The spectrum of $R$ is then the union of the diagonal elements of $T_u, T_d$ and the spectrum of $R_{scc}$. Now three options are possible. First, if $R^{ref}$, the spectral radius of $R$ and reference reproduction ratio, is among the diagonal elements of $T_d$ this means that there is one community that sustains the epidemic and at most exports cases to other sink communities (remember $T_d$ is lower diagonal), so it is a trivial case with no actual epidemic dynamics between communities.

Second, if $R^{ref}$ belongs to the spectrum of $R_{scc}$, then we shall write the Perron eigenvector in blocks as follows:

$$\mathbf{v} = \left(\begin{array}{c} \mathbf{v}_u \\ \hline \mathbf{v}_{scc} \\ \hline \mathbf{v}_d \end{array}\right). \tag{S2}$$

If we write by blocks the eigenvector equation $R\mathbf{v} = R^{ref}\mathbf{v}$, on the top block we have $T_u v_u = R^{ref} v_u$, whose only solution is $\mathbf{v}_u = 0$ as $R^{ref}$ is not an eigenvalue of $T_u$. This means $R_{scc}\mathbf{v}_{scc} = R^{ref}\mathbf{v}_{scc}$, and $\mathbf{v}_d = \left(R^{ref} - T_d\right)^{-1} B_3\mathbf{v}_{scc}$, this being nonsingular because $R^{ref}$ is not an eigenvalue of $T_d$. The dynamics is thus completely determined by the strongly connected component, and we can restrict our study to $R_{scc}$, which represents by definition a strongly-connected graph and as such is irreducible, proving our initial claim.

Finally, if $R^{ref}$ is among the diagonal elements of $T_u$ again this means that there is one community that generates cases and exports them, possibly through several steps, to the

strongly-connected component. Again this is seeding part is trivial and underlies no actual epidemic dynamics between communities, so that again we can restrict our study to $R_{scc}$.

## 1.2 Local estimated reproduction ratio

### 1.2.1 Convergence

We prove here that when the spatial distribution of infections is at equilibrium ($\mathbf{x} = \mathbf{v}$) and $r_i^{estim} = R^{ref}$, this implies a detailed balance between locally generated infections, imported infections and exported infections. First, we define the three quantities as computed from the previous generation:

$$I_i^{LOC}(t) = R_{ii} I_i(t-1); \tag{S3}$$

$$I_i^{IN}(t) = \sum_{j \neq i} R_{ij} I_j(t-1); \tag{S4}$$

$$I_i^{OUT}(t) = I_i(t-1) \sum_{j \neq i} R_{ji} = (\rho_i - R_{ii}) I_i(t-1). \tag{S5}$$

Clearly, $I_i(t) = I^{LOC}(t) + I^{IN}(t)$. But at the equilibrium is it also true that $I_i(t) = R I_i(t-1)$. Rewriting it as a function of $I^{OUT}(t)$ we can get to the detailed balance (omitting $t$):

$$I_i^{LOC} + I_i^{IN} = \frac{R^{ref}}{\rho_i - R_{ii}} I_i^{OUT}. \tag{S6}$$

### 1.2.2 Decay modes

It is possible to get an equivalent of equation (4) of the main paper to study the deviation of the local estimated reproduction ratio ($r_i^{estim}$) from $R^{ref}$. Defining $\Delta^{(i)}(t) = (r_i^{estim} - R^{ref})/R^{ref}$ as the relative difference, and proceeding analogously to $\Delta(t)$, one can simply replace $\mathbf{F}^T$ with $\mathbf{E}^{(i),T}$, the canonical basis covector which has 1 in $i$ and zero otherwise. This selects the specific community $i$ instead of summing over them as in the global case. Then

$$\Delta^{(i)}(t) = \frac{1}{R^{ref}} \frac{\mathbf{E}^{(i),T} R^t (R - R^{ref}) \mathbf{x}(0)}{\mathbf{E}^{(i),T} R^t \mathbf{x}(0)}. \tag{S7}$$

Proceeding, again, analogously to what described in the methods for $\Delta(t)$, one can get to

$$\Delta^{(i)}(t) = C^{(i)}(t) \sum_{\alpha} z_{\alpha}^{(i)} \left(1 - \frac{\Lambda_{\alpha}}{R^{ref}}\right) \left(\frac{\Lambda_{\alpha}}{R^{ref}}\right)^t, \tag{S8}$$

where $z_{\alpha}^{(i)} = -\mathbf{E}^{(i),T} \mathbf{w}_{\alpha} \mathbf{w}_{\alpha}^* \mathbf{x}(0)$ encode the weight of each mode. Comparing this with equation (4) and equation (12) of the main paper one notices that the local bias has the

same decay modes as the global ones (the eigenvalues of $\mathbf{R}$), but the weight of each mode is different in each community, and different from the global weight. Also, the global weight of each mode is the sum of the local weights: $z_\alpha = \sum_i z_\alpha^{(i)}$. Importantly, given that the weights $z_\alpha^{(i)}$ may are possibly complex numbers with negative real part and/or nonzero imaginary part (see also Methods of the main paper), this means the weights of modes that are dominant in some communities may cancel out making those modes negligible in determining the speed of convergence of the global estimated reproduction ratio. This means that, in some communities, $\Delta^{(i)}(t)$ may behave very differently from $\Delta(t)$. Specifically, oscillatory modes that are suppressed globally may dominate locally: even when oscillations are not globally visible, some $\Delta^{(i)}(t)$ may oscillate.

## 1.3 Estimation of department-level incident infections

In this section we describe the models used to estimate incident infections from incident hospitalizations in each department of mainland France (excluding Corsica), and compare them to serological estimates. COVID-19-related hospitalizations were collected and made available by the French health authorities and are available at `https://www.data.gouv.fr/en/datasets/donnees-hospitalieres-relatives-a-lepidemie-de-covid-19/`.

### 1.3.1 Models

In the main paper we did what we previously did in Ref. [2] and we reconstructed incident infections $I(d)$ from incident hospitalizations $H(d)$ as follows: $I(d) = H(d+7)/0.032$, where $0.032$ is the infection-hospitalization rate (IHR) and 7 is the average time from infection to hospitalization [3]. $d$ indicates the physical time in days.

We also tested an alternative approach featuring age stratification. We used two datasets for hospitalizations: i) department-level, non-age-stratified; ii) region-level, age-stratified. The French health authorities did not release department-level, age-stratified hospitalization data. Note: regions are made up of various departments. In mainland France (excluding Corsica) there are 12 regions and 94 departments. Age-stratification was available at the following age classes: $[0-9]$, $[10-19]$, $[20-29]$, $[30-39]$, $[40-49]$, $[50-59]$, $[60-69]$, $[70-79]$, 80 or older. We used age-stratified IHR for the same age classes from Ref. [4]. Finally, we got the number of residents of department $i$ in age class $a$ from the French national statistical institute (INSEE - `https://www.insee.fr`). Using the above data, we estimated the incidence of infections in each department of each region as follows. Given that our method applies independently to each region, we assume

in the following that we are focusing on a generic region and $i$ is the index running over the departments of that region, and we omit the index of the region. Analogously, we omit the time index $d$ as we can do the calculation at any time and then shift back by 7 days as we did in the former methodology. So let $H_a^{(reg)}$ be the number of incident hospitalizations in the region in age class $a$. Let $H_i^{(dep)}$ be the number of incident hospitalizations in department $i$ (non-age-stratified). Let $e_a$ be the IHR of age class $a$. Let $N_{ia}$ be the number of residents in department $i$ and age class $a$. With these ingredients, we define $f_{ia}$ as the fraction of individuals in age class $a$ and department $i$ who get infected (incident infections). We factor $f_{ia}$ as the product of a location term $c_i \geq 0$ and an age-class term $q_a \geq 0$, i.e., $f_{ia} = c_i q_a$, with the constraint $\sum_i c_i = 1$. Then, the frequency of individuals in age class $a$ in department $i$ getting hospitalized is $f_{ia}^{(h)} = e_a c_i q_a$. The following consistency equations must hold:

$$\begin{cases} \sum_i N_{ia} f_{ia}^{(h)} = H_a^{(reg)} \\ \sum_a N_{ia} f_{ia}^{(h)} = H_i^{(dep)} \end{cases} . \tag{S9}$$

Putting the expression of $f_{ia}^{(h)}$, we get

$$\begin{cases} e_a q_a \sum_i N_{ia} c_i = H_a^{(reg)} \\ c_i \sum_a N_{ia} e_a q_a = H_i^{(dep)} \end{cases} . \tag{S10}$$

We can solve equation (S10) numerically for $q_a, c_i$, with the only requirement of parametrizing $c_i$ as a unit simplex given the constraint $\sum_i c_i = 1$. This gives the daily estimated incidence of cases in each department as $c_i \sum_a N_{ia} q_a$.

We show in Fig. S8 alternative versions of Fig. 1**b** and Fig. 4 of the main paper, obtained using infections estimated with this methodology, proving that choosing either model (age-stratified vs non-age-stratified) gives the same findings.

### 1.3.2 Comparison to seroprevalence data

We found three studies estimating seroprevalence overall in France and in its regions in the period form 2020-03-10 to 2020-06-30 :

- *SpF*: from Ref. [5];
- *EpiCov*: from Ref. [6];
- *Carrat et al.*: from Ref. [7].

At the national level, we also compared our estimates (both non-age-stratified and age-stratified) with a model that we previously published [3]. We compared their estimates to the cumulative incidence estimated through our methodologies. See Fig. S5 for

the national estimate and Fig. S6 for the regional estimate. Interestingly, the reconstruction from non-age-stratified data (the one we use in the main manuscript) outperforms that from age-stratified data at the national level both according to the available serological estimates and our previous model. At the regional level, both perform generally well except for two regions (Grand-Est and Île-de-France) where the non-age-stratified reconstruction seems to overestimate infections. Also, in some regions, alternative serological studies may also give slightly incompatible estimates making it harder to assess which of our reconstructions schemes works better. In Provences-Alpes-Côte d'Azur, for instance, the non-age-stratified method is a better match to EpiCov, while the age-stratified one is a better match to Santé Publique France's. To investigate whether these regional variations may be associated with different age profiles in the resident population we calculated the proportion of residents older than 69 years old, and younger than 21 years old, by region: see Fig. S7. The result is inconclusive: the discrepancy in Île-de-France - the region of Paris, Île-de-France (IDF) in the maps below - indeed associates with the fact that the population there tends to be younger than the rest of France. But Grand-Est (GES in the map) has an age profile that is not substantially different from other regions where the non-age-stratified model does not overestimate infections. Analogoulsy, Provences-Alpes-Côte d'Azur (PAC in the map) has, for instance, an age profile similar to Occitanie (OCC) but the performance of the two estimation models is different: in PAC the age-stratified models seems to better reproduce SpF serological estimates, in OCC the EpiCov ones (the opposite for the non-age-stratified model), keeping in mind that differences between the two models are small anyways.

### 1.4 The stochastic epidemic model

We implement a discrete-time stochastic metapopulation model with an SEIR compartmental model, with a time step $\Delta d = 1\,day$. Let $S_i(d), E_i(d), I_i(d), R_i(d)$ be the number of residents of department $i$ in each compartment on day $d$. Being the population of each department fixed ($n_i$), the following continuity equation holds: $S_i(d) + E_i(d) + I_i(d) + R_i(d) = n_i \;\forall d$, where $n_i$ is the population in $i$. Let $\beta, \epsilon, \mu$ be the rates regulating the transitions $S \to E$, $E \to I$, $I \to R$. The latency and infectious periods are thus exponentially distributed with rates $\epsilon, \mu$: $\epsilon$ is the inverse of the average latency period and $\mu$ is the inverse of the average infectious period. One can then compute the probability of individual transition $E \to I$ in the discretization time step $\Delta d$ as the probability that the latency period is shorter than $\Delta d$: $p_\epsilon = 1 - e^{-\epsilon\Delta d}$. Analogously, the probability of individual recovery is $p_\mu = 1 - e^{-\mu\Delta d}$. $\beta$ is the parameter regulating transmissibility. Let $p_{ij}$ be the colocation

matrix, then the individual rate of becoming infected is $\beta \sum_j p_{ij} I_j(d)$ – see Ref. [8]. And as before the probability of individual infection is $p_{\beta,i}(d) = 1 - e^{-\beta \sum_j p_{ij} I_j(d) \Delta d}$.

We now describe the $d$-th time step of the algorithm to compute $E_i(d), I_i(d), R_i(d)$ from $E_i(d-1), I_i(d-1), R_i(d-1)$, using the probabilities just computed:

- sample $E_i^{(S\to E)} \sim \text{Binom}\,(n = S_i(d-1), p = p_{\beta,i}(d))$;
- sample $I_i^{(E\to I)} \sim \text{Binom}\,(n = E_i(d-1), p = p_\epsilon)$;
- sample $R_i^{(I\to R)} \sim \text{Binom}\,(n = I_i(d-1), p = p_\mu)$;
- update $E_i(d) = E_i(d-1) + E_i^{(S\to E)} - I_i^{(E\to I)}$;
- update $I_i(d) = I_i(d-1) + I_i^{(E\to I)} - R_i^{(I\to R)}$;
- update $R_i(d) = R_i(d-1) + R_i^{(I\to R)}$.

### 1.4.1 Reference reproduction ratio

The deterministic continuous-time ordinary differential equations of this model are

$$\begin{cases} \dot{E}_i = \beta S_i \sum_j p_{ij} I_j - \epsilon E_i \\ \dot{I}_i = \epsilon E_i - \mu I_i \\ \dot{R}_i = \mu I_i \end{cases} \tag{S11}$$

In the notation of the next-generation-matrix formalism [9]

$$\begin{cases} \dot{E}_i = \mathcal{F}_i^E - \mathcal{V}_i^E \\ \dot{I}_i = \mathcal{F}_i^I - \mathcal{V}_i^I \\ \dot{R}_i = \mathcal{F}_i^R - \mathcal{V}_i^R \end{cases} \tag{S12}$$

with $\mathcal{F}_i^E = \beta S_i \sum_j p_{ij} I_j$, $\mathcal{F}_i^I = \mathcal{F}_i^R = 0$, $\mathcal{V}_i^E = \epsilon E_i$, $\mathcal{V}_i^I = \mu I_i - \epsilon E_i$ and $\mathcal{V}_i^R = -\mu I_i$. Then we define the $2N \times 2N$ block matrices matrices $F, V$:

$$F = \left( \begin{array}{c|c} \frac{\partial \mathcal{F}_i^E}{\partial E_j} & \frac{\partial \mathcal{F}_i^E}{\partial I_i} \\ \hline \frac{\partial \mathcal{F}_i^I}{\partial E_j} & \frac{\partial \mathcal{F}_i^I}{\partial I_i} \end{array} \right)_{E=I=R=0} = \left( \begin{array}{c|c} 0 & \beta n_i p_{ij} \\ \hline 0 & 0 \end{array} \right) \tag{S13}$$

$$V = \left( \begin{array}{c|c} \frac{\partial \mathcal{V}_i^E}{\partial E_j} & \frac{\partial \mathcal{V}_i^E}{\partial I_i} \\ \hline \frac{\partial \mathcal{V}_i^I}{\partial E_j} & \frac{\partial \mathcal{V}_i^I}{\partial I_i} \end{array} \right)_{E=I=R=0} = \left( \begin{array}{c|c} \epsilon \delta_{ij} & 0 \\ \hline -\epsilon \delta_{ij} & \mu \delta_{ij} \end{array} \right). \tag{S14}$$

So, by the next-generation-matrix theory:

$$NGM_{ij} = \left(FV^{-1}\right)_{ij} = \frac{\beta}{\mu} n_i p_{ij}. \tag{S15}$$

Given our reconstruction of $\mathbf{R}$ from the colocation matrix (see Methods, Reconstruction of the reproduction operator from data) one can see that $R_{ij} = NGM_{ij}$ if $C = \beta/\mu$, building the final connection between our theoretical formalism and the stochastic simulations. Specifically, the equivalence between the reference reproduction ratio in our calculations and that of the stochastic model: $R^{ref} =$ spectral rad$(NGM)$.

### 1.4.2 Generation interval and EpiEstim settings

The generation interval is the time between infection and subsequent transmission to another individual. Estimating $R$ through the R-package EpiEstim requires feeding the generation interval distribution associated to the disease[10]. We obtain here the generation interval for our epidemic model.

The compartmental model we use (see Methods and Ref. [11]) has a rate of transition from the E to the I compartment ($\epsilon$) and a recovery rate $\mu$. We also define an effective transmissibility $\mu R^{ref}$ (see equation (15) of main paper). Let $\tau$ be the generation time. Let the probability that a transmission event occurs exactly after $\tau$ has passed since primary infection be $P(t)dt$. Also, let $\tau_E$ be the time one stays in the E compartment: $\tau_E \sim$ Exp$(\epsilon)$, and $\tau_I$ be the time one stays in the I compartment: $\tau_I \sim Exp(\mu)$. Conditioning on $\tau_E, \tau_I$, we have

$$P(\tau|\tau_E, \tau_I)dt = \mu R^{ref} dt \theta(\tau - \tau_E)\theta(\tau_I + \tau_E - \tau), \tag{S16}$$

where $\theta$ is the Heaviside's function. So now we marginalize and get the generation time distribution $P(\tau)$:

$$P(\tau) = \int_0^\infty d\tau_E d\tau_I P(\tau|\tau_E, \tau_I)P(\tau_E)P(\tau_I) = \frac{\mu\epsilon R^{ref}}{\mu - \epsilon}\left(e^{-\epsilon\tau} - e^{-\mu\tau}\right). \tag{S17}$$

Note that a discrete distribution is required by the EpiEstim package. We choose to compute it over 50 bins in the interval $[0, 49]$. The time window over which to estimate $R$ is set to be a week. In all simulations, we assign the estimate for $R$ returned for the week interval $[t, t+6]$ to the day $t+3$. Also, given the smaller precision of early estimates, as reported in the documentation [10], we arbitrarily choose not to plot EpiEstim points associated to the first two weeks from the start of the synthetic epidemic.
For all figures shown in the main manuscript and Supplementary Information, we run multiple runs of the model and compute the reproduction ratio from incident infections produced in each of the runs (according to the framework described in the main paper, with EpiEstim, or both). We show point-wise medians computed over runs and 95%

confidence intervals as statistics of the results. In Fig. S10 and Fig. S11 we show a comparison between so obtained point-wise medians with confidence intervals, and examples of single runs of the stochastic model, in order to test their qualitative match.

## 1.5 Oscillations in European countries

We included 32 European countries: 24 members of the European Union (excluding Cyprus, Ireland and Latvia for lack of data) plus Albania, Bosnia and Herzegovina, Iceland, Montenegro, Norway, Serbia, Sweden, UK (see Data availability). For all of them we built the operator $R$ using colocation and population data at the admin-2 level, similarly to what we did for France. We found at least one real, negative eigenvalue in 11 out of 32 countries, but nowhere did they cause visible oscillations, as the oscillation period was always larger than twice the decay time (Fig. S1). We did not find nonreal eigenvalues. This begs the question whether oscillations are actually observable in real systems. To rigorously determine the conditions for a specific spectrum in a generic nonnegative matrix is not possible, except for specific or low-dimensional cases [12]. We can, however, plausibly associate the presence of an oscillating mode with period $T_\alpha$ to the existence of a cycle of approximate length $T_\alpha$ in the (weighted, directed) network which has $R$ as its adjacency matrix [13, 14]. Slow oscillations (large $T_\alpha$) would then require the presence of long cycles in $R$, which are unlikely to be generated by the recurrent mobility patterns that drive the spatial spread of epidemic outbreaks following pathogen importation [15, 16]. Fast oscillations, and in particular those generated by real, negative eigenvalues, may instead be more common. They would require epidemics that are strongly coupled, i.e., where pairs of communities exist in which infected residents generate, on average, more infections in the other community than in their own, but this is not the case in the countries we examined and for the spatial resolution we considered.

# 2 Supplementary Figures

## 2.1 Decay time and oscillation period of the modes of $\Delta = R^{estim} - R^{ref}$ for selected European countries

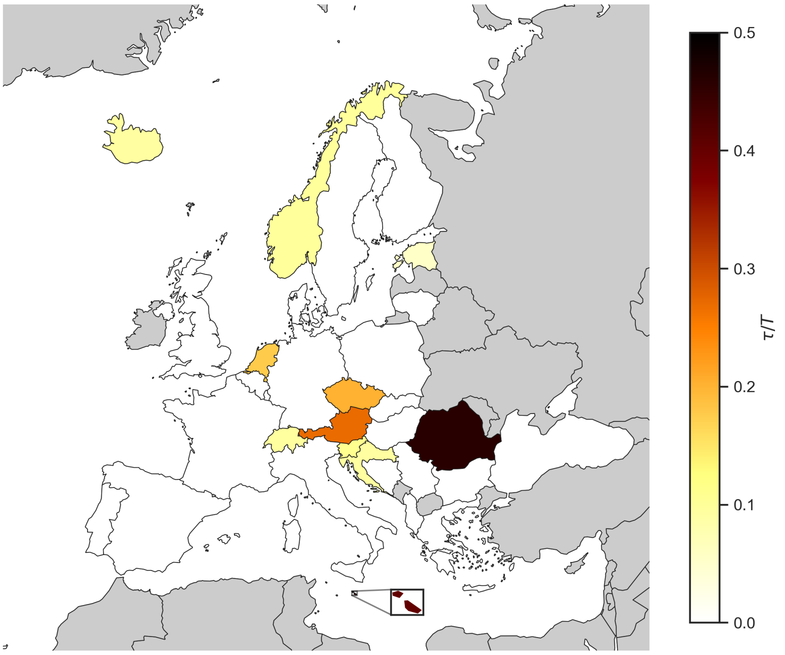


**Fig.S1**|**Decay time and oscillation period of the modes of $\Delta = R^{estim} - R^{ref}$ for selected European countries.** The color shows the value, for each country, $\max_\alpha \tau_\alpha / T_\alpha$, where $\tau_\alpha, T_\alpha$ are defined in the main paper and are, respectively, the decay time and the oscillation period of the $\alpha$th mode. 32 countries are included: 24 members of the European Union (excluding Cyprus, Ireland and Latvia for lack of data) plus Albania, Bosnia and Herzegovina, Iceland, Montenegro, Norway, Serbia, Sweden, UK (see Data availability). Countries with real positive eigenvalues only are colored in white ($T_\alpha = \infty$), countries not included are in gray.

## 2.2 Relative effect of the diagonal correction to co-location probabilities in French departments

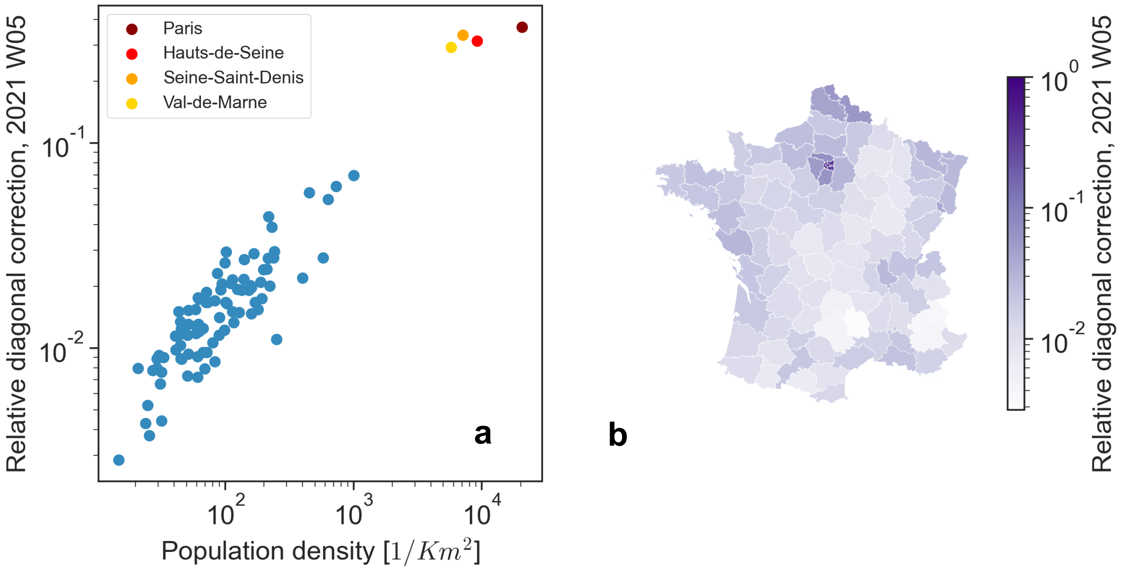


**Fig.S2**|**Relative effect of the diagonal correction to co-location probabilities in French departments.** **a** shows the relative effect of the diagonal corrections in the 94 departments of mainland France in week 5 of 2021, with respect to population densities. The correction is substantial in departments with high population density, consistently with the nature of the bias we want to correct. See Methods, Reconstruction of the reproduction operator from data. **b** map of the relative diagonal corrections.

## 2.3 Daily number of new COVID-19-related infections per 100,000 residents

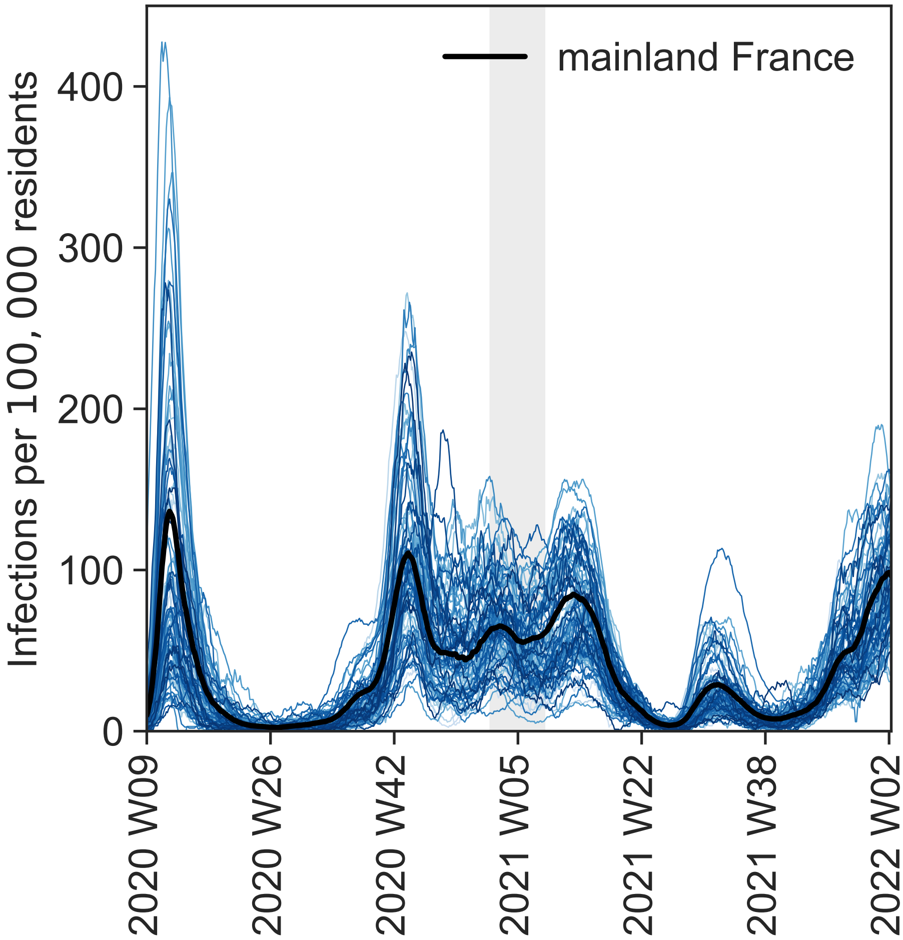


**Fig.S3|Daily number of new COVID-19-related infections per 100,000 residents**. Daily incident infections from week 9 of 2020 to week 3 of 2022 (Feb 23, 2020 to Jan 23, 2022), according to the estimation method we use in the main paper. Each curve is that of one of the 94 departments (administrative level 2) of mainland France excluding the region of Corsica, with a 14 days window rolling average. The area in gray goes from week 2 to week 9 of 2021 (Jan 11 to Mar 7), corresponding to the period on which we focus in Fig. 1 of the main paper. The small Dept. #90 (Territoire de Belfort), containing 0.2% of the French population, is excluded for visibility as it had an anomalously high estimated incidence peaking at around 600 due to a miscounting of hospitalizations coming from neighboring departments. This fact was known to national health authorities.

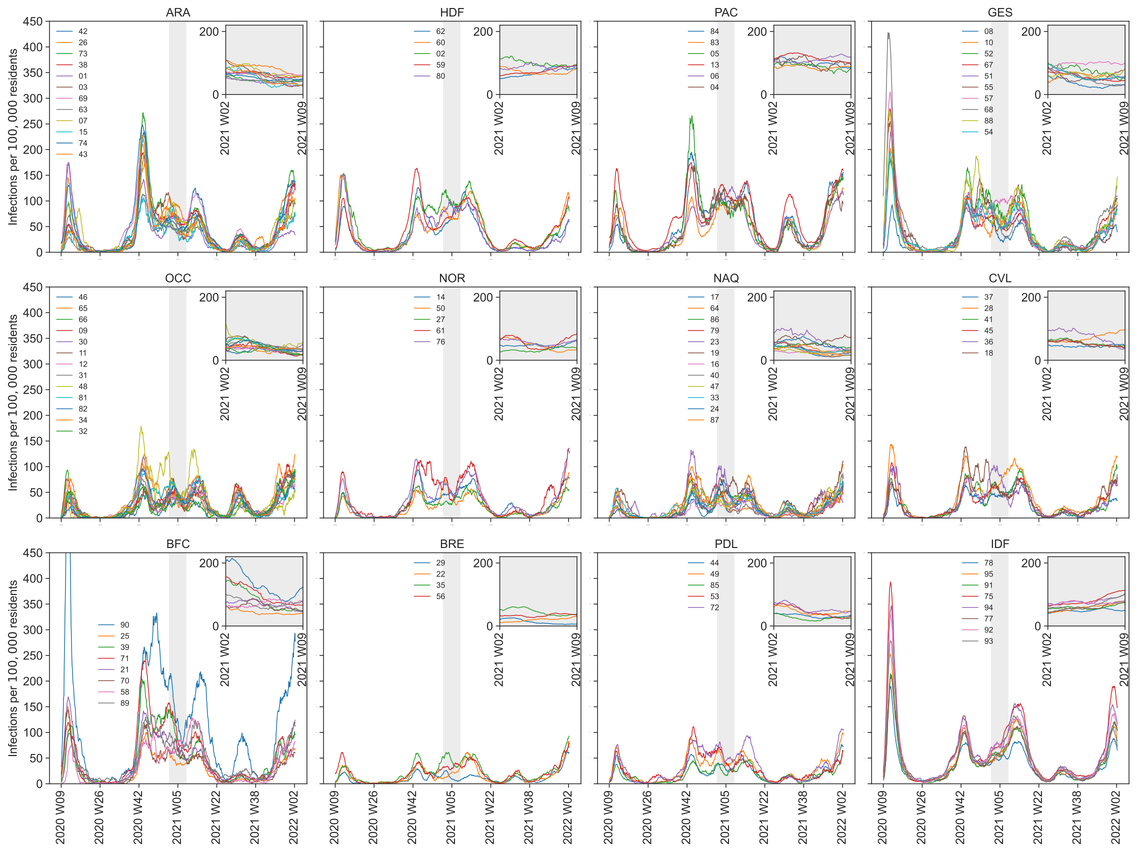


**Fig.S4**|**Daily number of new COVID-19-related infections per 100,000 residents in the 12 regions of mainland France.** We show new COVID-19-related daily infections estimated according to the method used in the main paper, separately for the departments in each of the twelve regions of mainland France, to facilitate readability. Names of regions (three letters codes) are reported in plot titles, while INSEE codes of departments are reported in the legend. Insets zoom in on the period from week 2 of 2021 to week 9 of 2021, the focus in Fig. 1 of the main paper. A 14 days window rolling average is used. The small Dept. #90 (Territoire de Belfort) in region Bourgogne-Franche-Comté (BFC), containing 0.2% of the French population, had an anomalously high estimated incidence peaking at around 600 due to a miscounting of hospitalizations coming from neighboring departments. This fact was known to national health authorities.

## 2.4 National attack rate: estimates vs serological studies

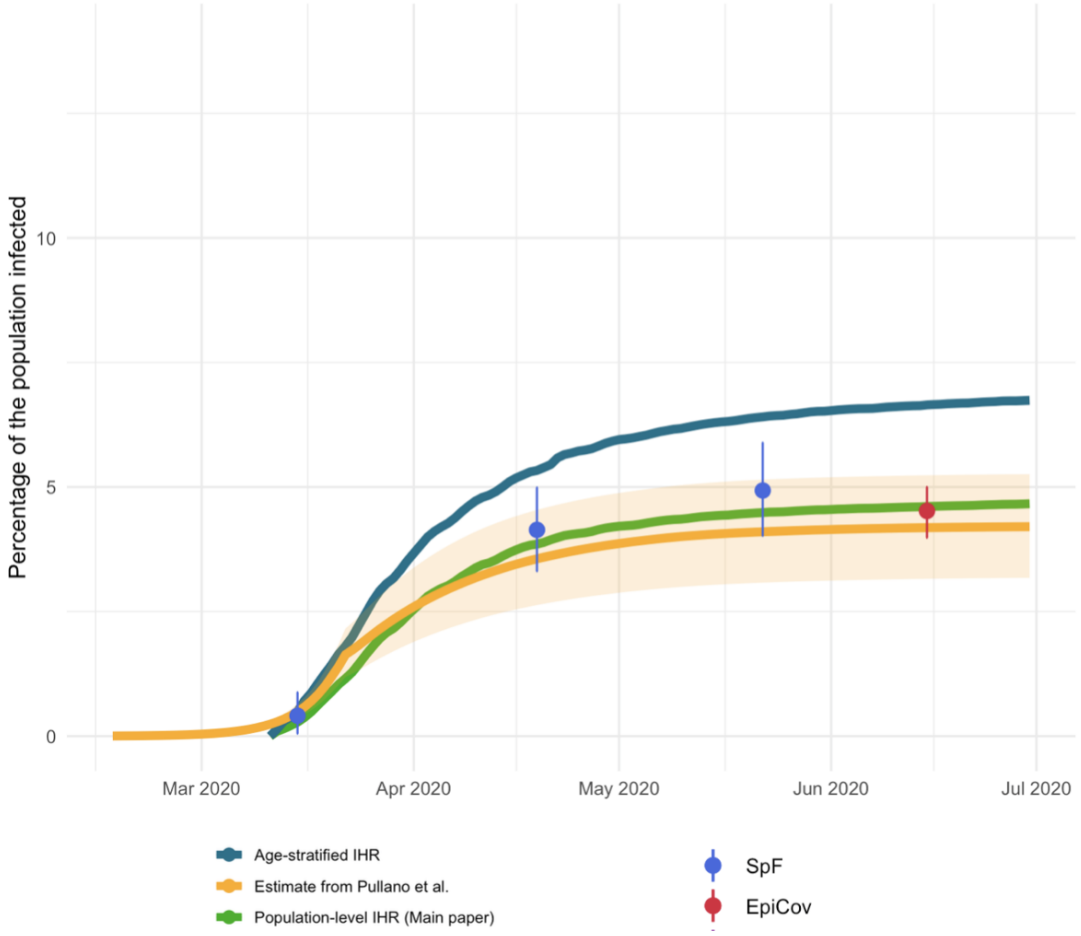


**Fig.S5|National attack rate: estimates vs serological studies.** This figure presents the cumulative attack rate across whole France, as per non-age-stratified estimation, age-stratified estimation, Pullano et al. estimation ([3]) and serological studies from SpF ([5]), EpiCov ([6]), and Carrat et al. ([7]). The estimates are plotted over time for the period from April to June 2020.

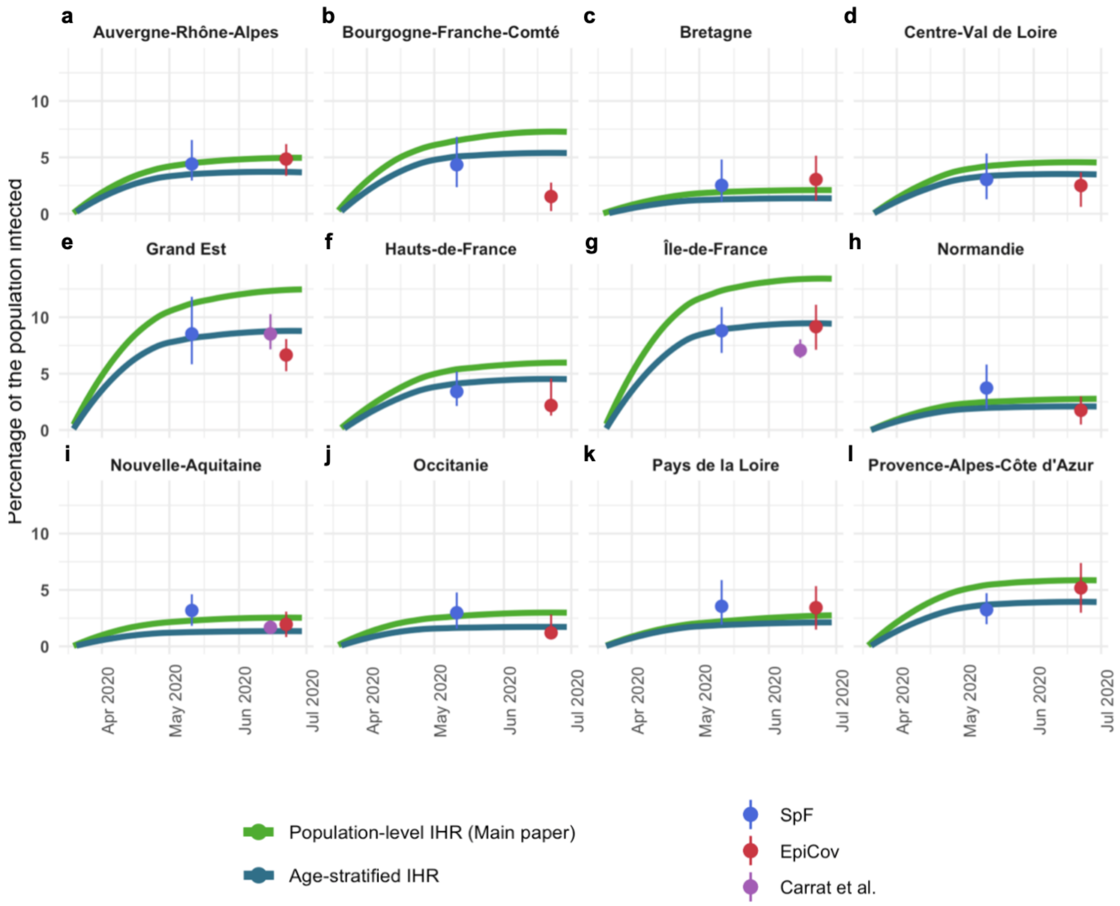


**Fig.S6|Regional attack rate: estimates vs serological studies.** This figure presents the cumulative attck rate across different French regions, as per the non-age-stratified estimation, age-stratified estimation, and serological studies from SpF ([5]), EpiCov ([6]), and Carrat et al. ([7]). The estimates are plotted over time for the period from April to June 2020.

## 2.5 Age demographic distribution in French regions

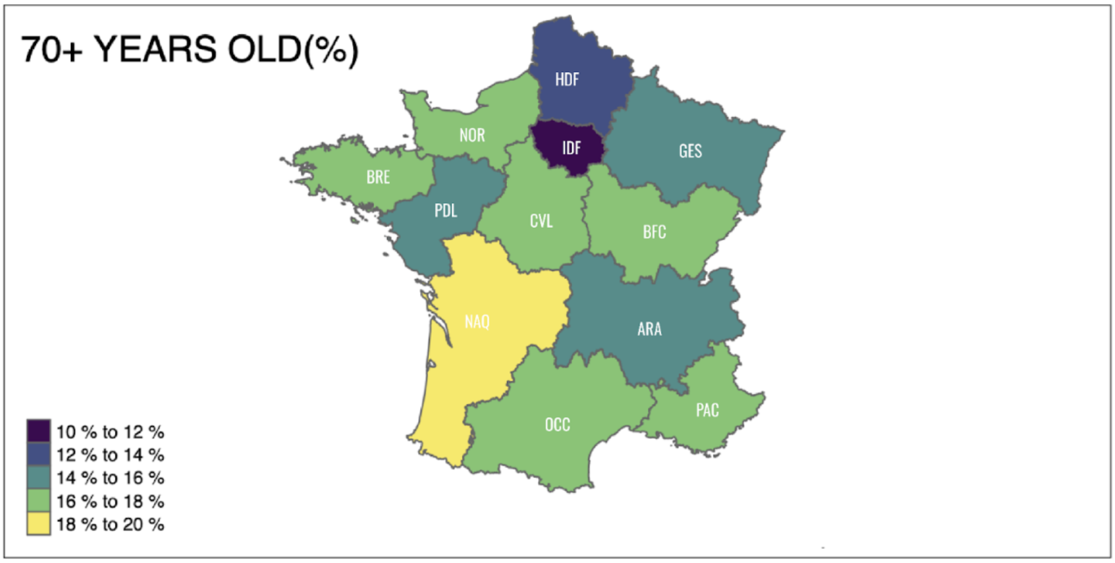


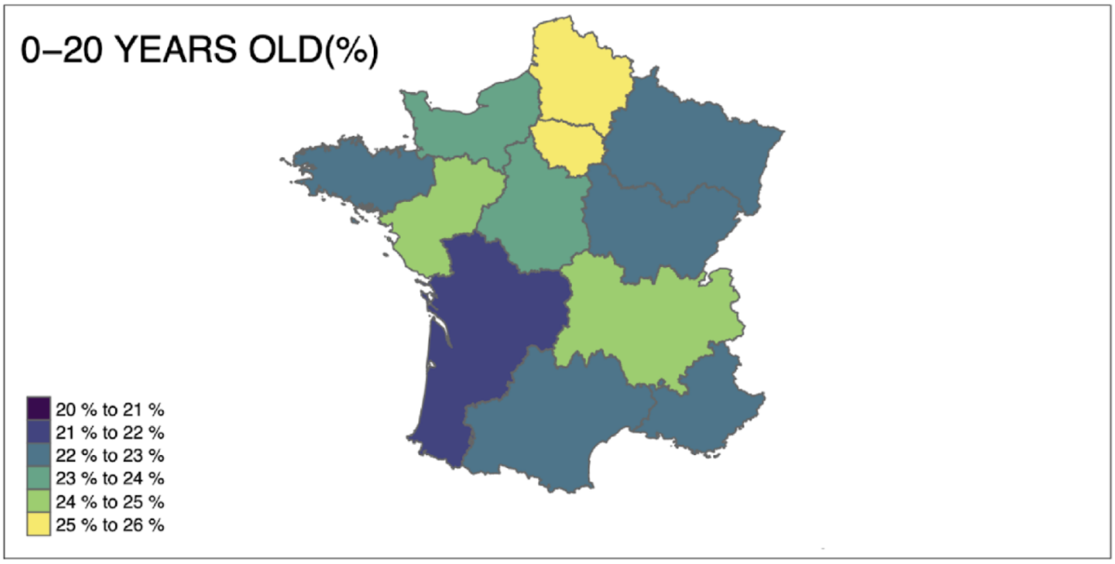


**Fig.S7|Age distribution in French regions.** The top map shows the percentage of the resident population aged 70 and above, while the bottom map details the percentage of the population aged 0 to 20.

## 2.6 Fig. 1b and Fig. 4 of the main paper, using the age-stratified model for the estimate of infections

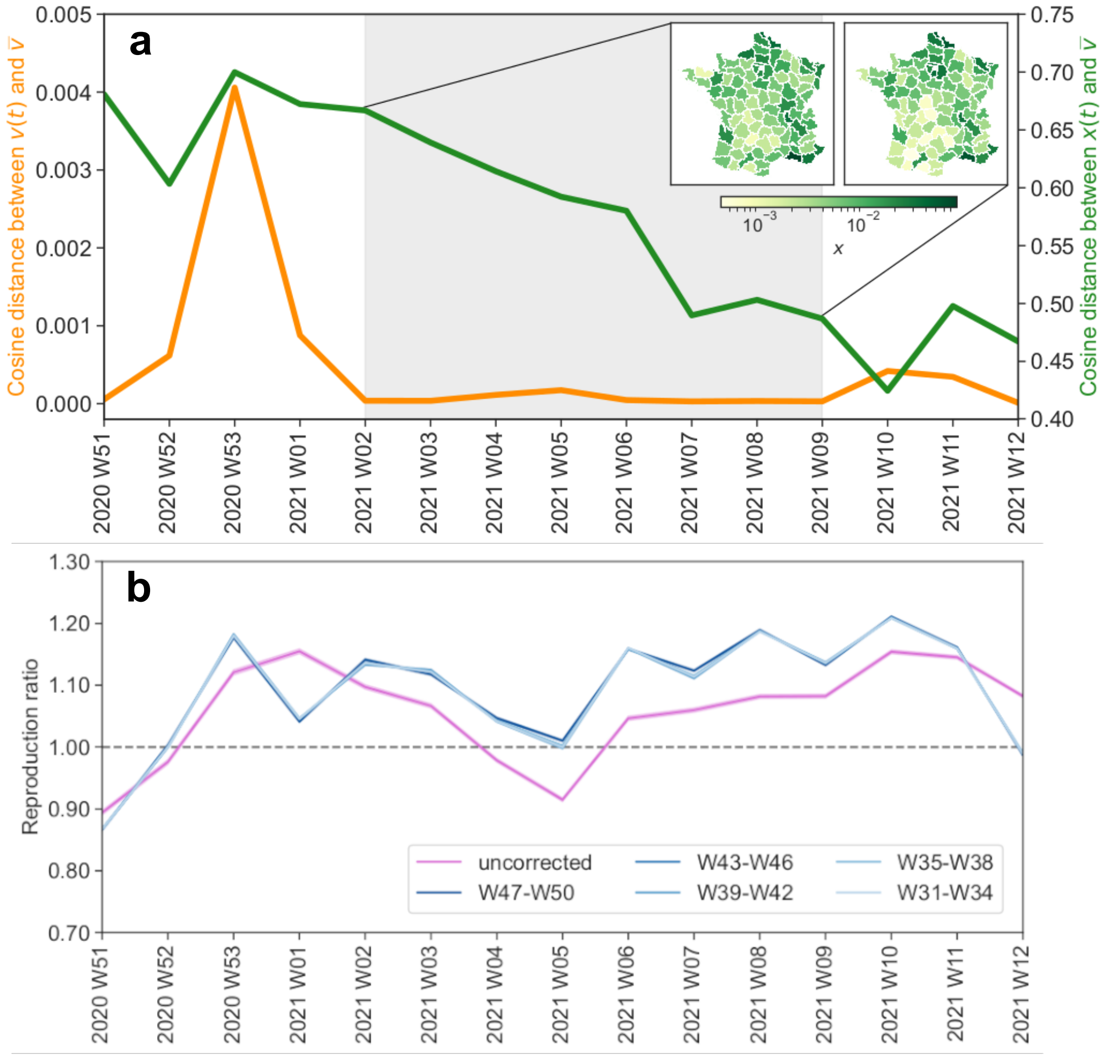


**Fig.S8**|**Fig. 1b and Fig. 4 of the main paper, using the age-stratified model for the estimate of infections.** We show an alternative version of Fig.1**b** and Fig.4 of the main paper, respectively in **a** and **b**. Here we consider new COVID-19 infections reconstructed as per the age-stratified model described in Estimation of department-level incident infections. Results are in agreement with the discussion related to Fig. 1**b** and Fig. 4 in the main paper. Also, we stress that the validity of our theoretical results is independent of the methodology employed for cases reconstruction.

## 2.7 Comparison of the reference, estimated and corrected reproduction ratios with six different initial conditions for the stochastic model

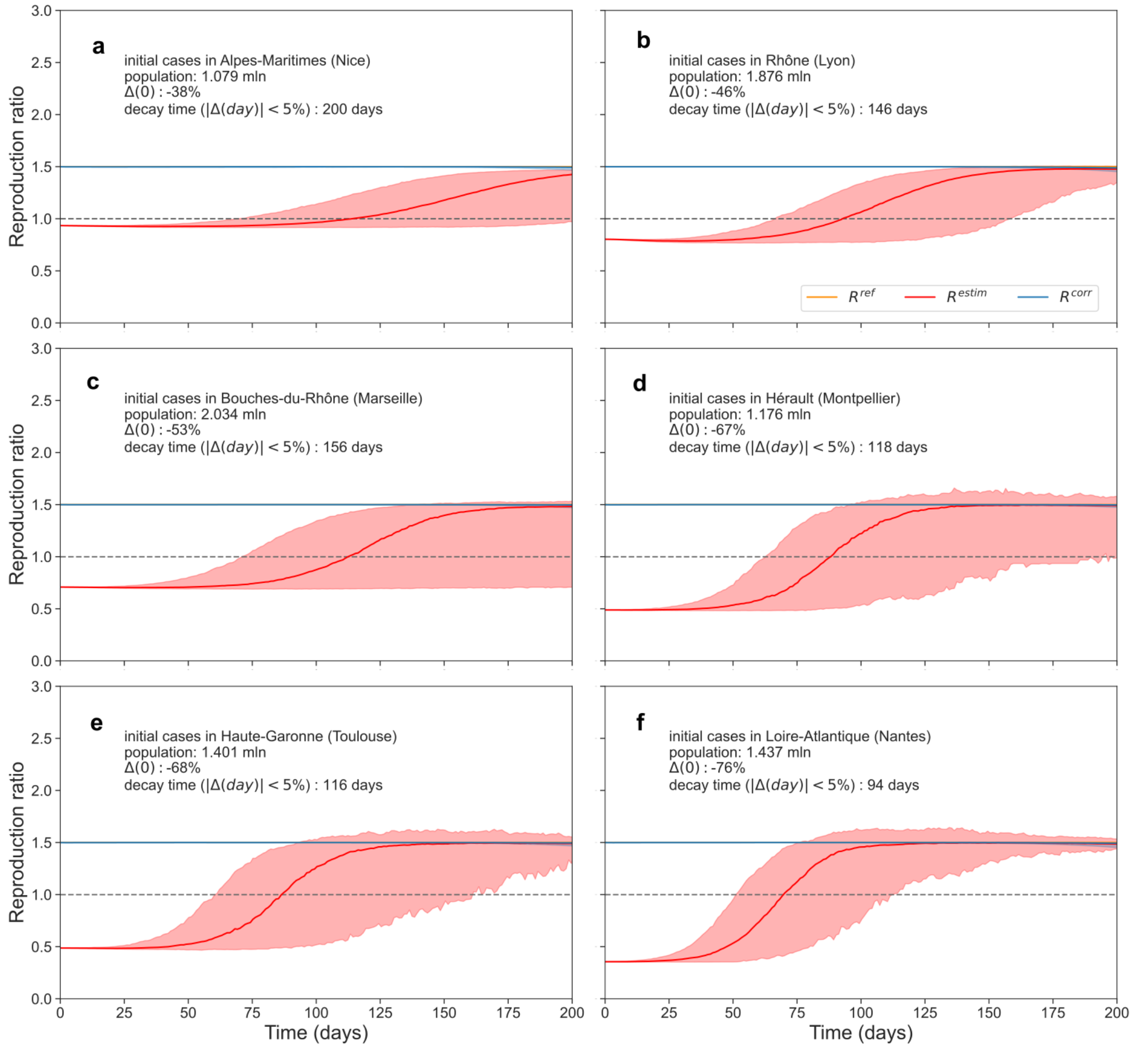


**Fig.S9**|**Comparison of the reference, estimated and corrected reproduction ratios with six different initial conditions.** This figure uses the same stochastic epidemic model as in Fig. 2 and Fig. 3 of the main paper, with six different initial conditions. 500 initial cases are seeded in Alpes-Maritimes (**a**), Rhône (**b**), Bouches-du-Rhône (**c**), Hérault (**d**), Haute-Garonne (**e**) and Loire-Atlantique (**f**). The largest city in each of these departments is written in parenthesis in legend, together with the departments' population, the initial (day=0) relative difference between the estimated and reference reproduction ratios, and the time in days required for the absolute relative error to be smaller than 0.05. Both the initial measurement error and the speed of convergence depend on the initial conditions, as discussed in the main paper. We show medians and 95% confidence intervals for reproduction ratios over 1,000 runs.

## 2.8 Comparison between point-wise medians and single runs of the stochastic metapopulation model

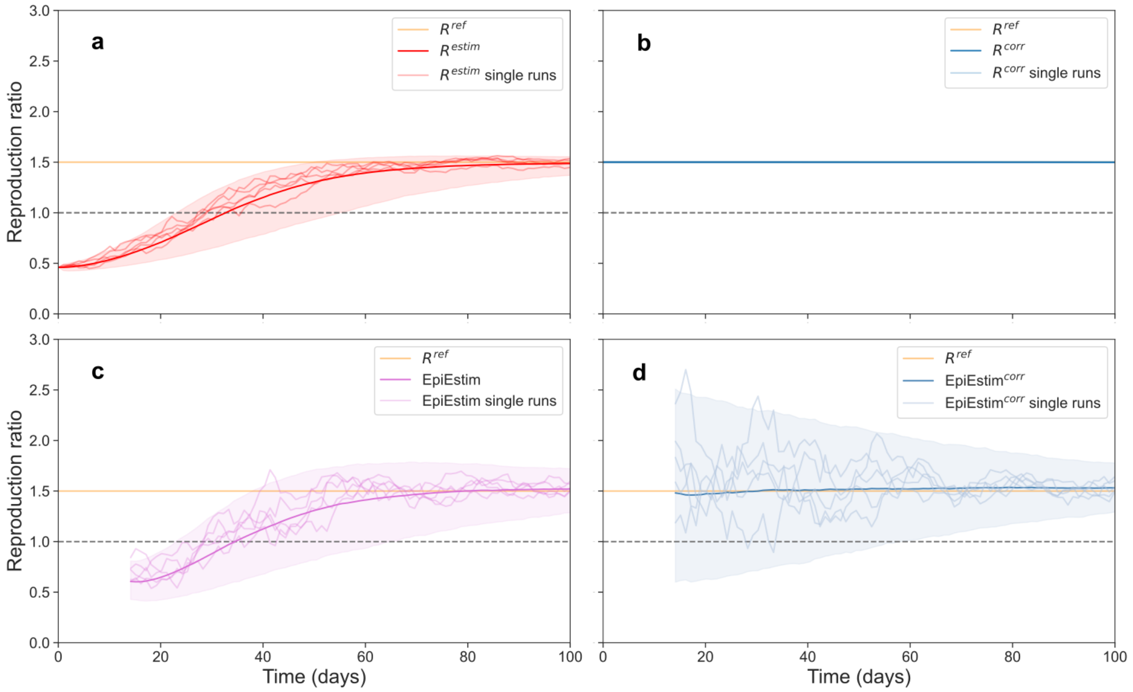


**Fig.S10|Comparison between point-wise medians and single runs of the stochastic model: estimates of the reproduction number.** This figure uses the same stochastic epidemic model as in Fig. 2 and Fig. 3 of the main paper, and one of their two initial conditions, *i.e.* 100 initial cases are seeded among departments proportionally to their population. We show the standard reproduction ratio measured from surveillance data – both in the Galton-Watson formalism (red, **a**) and with *EpiEstim* (purple, **c**) on incidence data – and the corresponding $\mathbf{v}^*$-corrected estimates: Galton-Watson formalism (blue, **b**) and with *EpiEstim* (light blue, **d**) on modified incidence data. We show point-wise medians and confidence intervals over $10,000$ runs, and we compare them with the results of single runs of the model, in order to test their qualitative match.

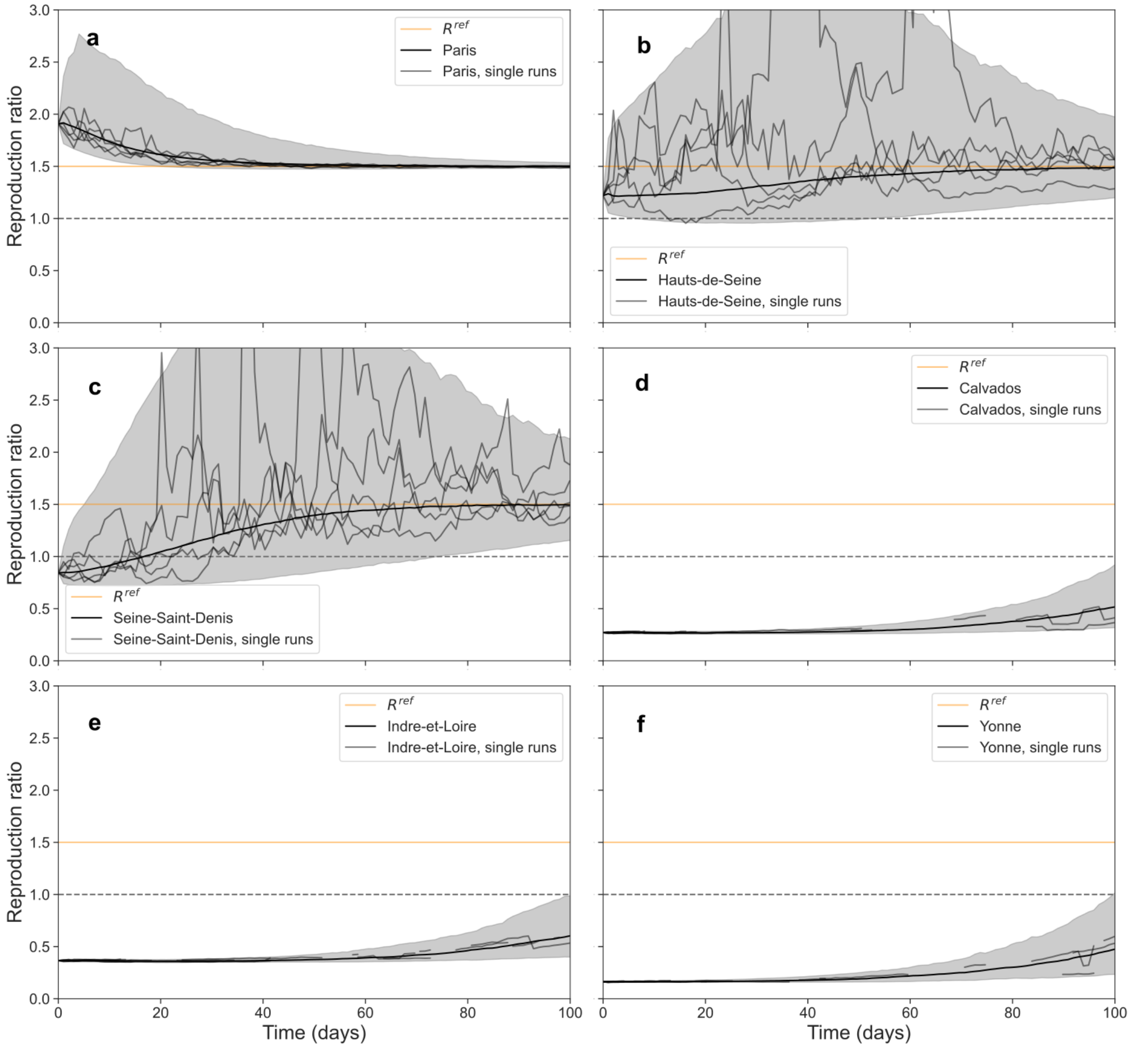


**Fig.S11|Comparison between point-wise medians and single runs of the stochastic model: locally estimated reproduction numbers.** This figure uses the same stochastic epidemic model as in Fig. 2 and Fig. 3 of the main paper, and one of their two initial conditions, *i.e.* 100 initial cases are seeded among departments proportionally to their population. We show the locally estimated reproduction numbers in 6 among the 94 departments of mainland France, which we report in the legend of single plots (**a**, **b**, **c**, **d**, **e**, **f**). We show point-wise medians and confidence intervals over $10,000$ runs, computed excluding points associated to locally extinct runs. Time points in which local incidence is zero are omitted.

## 2.9 Variation of the spatial distribution of infections between weeks 6 and 11 of 2021, and the equilibrium distribution

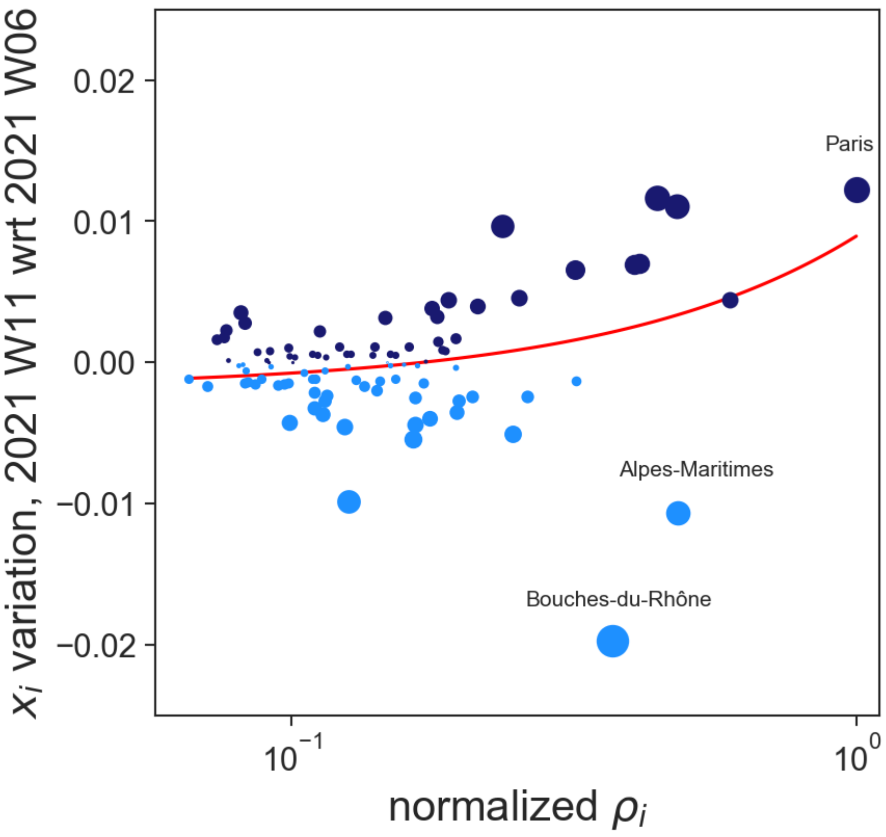


**Fig.S12|Variation of the spatial distribution of infections between weeks 6 and 11 of 2021, against the transmission potential of communities.** We show on the x axis the transmission potential of each department (rescaled so that the highest equals one) and on the y axis the difference between the fraction of national infections in that department in Week 6 and 11 of 2021. Departments with high transmission rates tended to increase their fraction of total infections, departments with low transmission rates tended to decrease it. The red line is a simple linear fit to help underline the trend. This is the overall trend, yet some departments still had their share of infections decrease even if they had a fairly high $\rho$ (the departments of the cities of Nice, Alpes-Maritimes, and Marseille, Bouches-du-Rhône, in the South of France). This is consistent with the values of these departments in the equilibrium spatial distribution of infections shown in Supplementary Fig. S13.

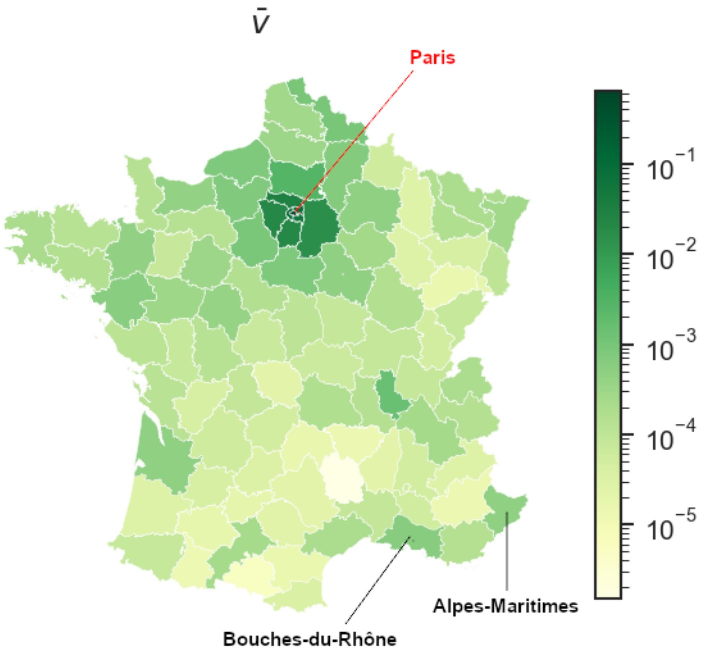


**Fig.S13**|**Equilibrium distribution of infections computed from the average reproduction operator between week 51 of 2020 and week 12 of 2021.** We show the average equilibrium distribution of infections in the time window of Fig. 1**b** and Fig. 4 of the main paper. Consistently with the known centrality of Paris in the French mobility network, the equilibrium distribution has high values in Île-de-France. The depatrments of Paris, Alpes-Maritimes and Bouches-du-Rhône are highlihgted with arrows, following the discussion of Supplementary Fig. S12.

# Supplementary References


1. Horn, R. A. & Johnson, C. R. *Matrix Analysis* ISBN: 0-521-38632-2 (Cambridge University Press, 1990).
2. Mazzoli, M., Valdano, E. & Colizza, V. Projecting the COVID-19 epidemic risk in France for the summer 2021. *Journal of Travel Medicine* **28.** ISSN: 1708-8305 (Oct. 2021).
3. Pullano, G. *et al.* Underdetection of COVID-19 cases in France threatens epidemic control. *Nature* **590** (Feb. 2021).
4. Le Vu, S. *et al.* Prevalence of SARS-CoV-2 antibodies in France: results from nationwide serological surveillance. en. *Nature Communications* **12.** Number: 1 Publisher: Nature Publishing Group, 3025. ISSN: 2041-1723 (May 2021).
5. Le Vu, S. *et al.* Prevalence of SARS-CoV-2 antibodies in France: results from nationwide serological surveillance. *Nature communications* **12,** 3025 (2021).
6. Ministère des Solidarités et de la Santé. *En mai 2020, 4,5% de la population en France métropolitaine a développé des anticorps contre le SARS-CoV-2. Premiers résultats de l'enquête nationale EpiCov* Accessed: 2023-11-29. 2020.
7. Carrat, F. *et al.* Antibody status and cumulative incidence of SARS-CoV-2 infection among adults in three regions of France following the first lockdown and associated risk factors: a multicohort study. *International journal of epidemiology* **50,** 1458–1472 (2021).
8. Iyer, S. *et al.* Large-scale measurement of aggregate human colocation patterns for epidemiological modeling. *Epidemics* **42,** 100663. ISSN: 1755-4365 (2023).
9. Diekmann, O., Heesterbeek, J. & Roberts, M. The construction of next-generation matrices for compartmental epidemic models. *Journal of the Royal Society, Interface / the Royal Society* **7,** 873–85 (Nov. 2009).
10. Cori, A., Ferguson, N. M., Fraser, C. & Cauchemez, S. A New Framework and Software to Estimate Time-Varying Reproduction Numbers During Epidemics. *American Journal of Epidemiology* **178,** 1505–1512. ISSN: 0002-9262 (Nov. 2013).
11. Faucher, B. *et al.* Agent-based modelling of reactive vaccination of workplaces and schools against COVID-19. *Nature Communications* **13,** 1414 (Mar. 2022).
12. Egleston, P. D., Lenker, T. D. & Narayan, S. K. The nonnegative inverse eigenvalue problem. en. *Linear Algebra and its Applications. Special Issue on the Tenth ILAS Conference (Auburn, 2002)* **379,** 475–490. ISSN: 0024-3795 (Mar. 2004).

13. Kellogg, R. B. & Stephens, A. B. Complex eigenvalues of a non-negative matrix with a specified graph. en. *Linear Algebra and its Applications* **20,** 179–187. ISSN: 0024-3795 (Jan. 1978).

14. Torre-Mayo, J., Abril-Raymundo, M. R., Alarcia-Estévez, E., Marijuán, C. & Pisonero, M. The nonnegative inverse eigenvalue problem from the coefficients of the characteristic polynomial. EBL digraphs. en. *Linear Algebra and its Applications* **426,** 729–773. ISSN: 0024-3795 (Oct. 2007).

15. Schneider, C. M., Belik, V., Couronné, T., Smoreda, Z. & González, M. C. Unravelling daily human mobility motifs. *Journal of the Royal Society Interface* **10.** ISSN: 17425662 (2013).

16. Gómez-Gardeñes, J., Soriano-Paños, D. & Arenas, A. Critical regimes driven by recurrent mobility patterns of reaction–diffusion processes in networks. en. *Nature Physics* **14.** Number: 4 Publisher: Nature Publishing Group, 391–395. ISSN: 1745-2481 (Apr. 2018).
